# Supplementary material for: SVEva Fair: A Framework for Evaluating Fairness in Speaker Verification
Source: arXiv:2107.12049 source file (2022-10-04)
Supplement: Supplementary file 1 [file appendix.tex]

\section{Appendix}
\label{appendix}

\begin{figure*}[hbt]
    \centering
    \subfigure[False negative weighted (10:1)]{
        \includegraphics[width=0.45\textwidth]{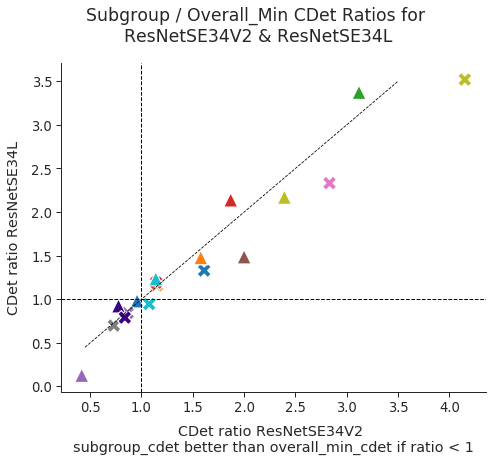}
        \label{fig:cdet_ratios_models_fnweighted}
    }
    \subfigure[False positive weighted (10:1)]{
        \includegraphics[width=0.52\textwidth]{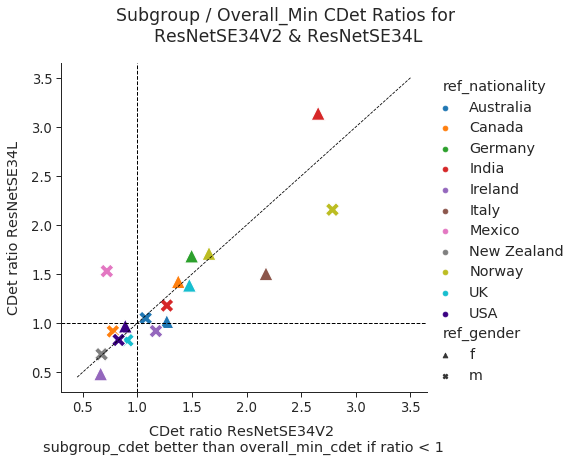}
        \label{fig:cdet_ratios_models_fpweighted}
    }
    \caption{Comparison of CDet ratios for subgroups at 10:1 weightings of false negative (left) and false positive (right) error rates for ResNetSE34V2 and ResNetSE34L models.}
\end{figure*}
